# Supplementary material for: Stabilization of singularly perturbed networked control systems over a single channel
Source: arXiv:2502.18768 source file (2025-02-26)
Supplement: Supplementary file 2 [file Appendix_Stable_fast_subsystem.tex]

\section{Proof of Corollary \ref{Corollary Stable fast subsystem}}

Assumptions \ref{Assumption reduced model}, \ref{Assumption interconnection} and \ref{Assumption Extra 2} are written for a more general model (i.e., $\mathcal{H}_2^y$), when we apply them to a specialized model with lower dimension, we ignore the states that does not exist in the specialized model. \cyan{For instance, $\mathcal{H}_5$ does not have the state $e_f$, then when we apply Assumption \ref{Assumption reduced model} to it, $f_x(x, \overline{H}(x,e_s),e_s,0)$ is replaced by $f_x(x, \overline{H}(x,e_s),e_s)$.} 
At the same time, Lemma \ref{Lemma MATI} is applicable to any reduced and boundary layer system with the same form as $\mathcal{H}_r$ and $\mathcal{H}_{bl}$. Since $\mathcal{H}_{5,r}$ has the same form as $\mathcal{H}_r$ and  Assumption \ref{Assumption reduced model} holds, we can conclude inequalities in \eqref{eqn: Us} hold, with $\mathcal{C}_{2,r}^{y,0}$ and $\mathcal{D}_{2,r}^{y,0}$ replaced by $\mathcal{C}_5^y$ and $\mathcal{D}_{5,s}^y$, respectively.
 %
%Since $\mathcal{H}_{5,r}$ has the same form as $\mathcal{H}_r$, Assumption \ref{Assumption reduced model} is applicable to $\mathcal{H}_{5,r}$, then by Lemma \ref{Lemma MATI}, there exist $U_s$ satisfies inequalities in \eqref{eqn: Us} with $\mathcal{C}_{2,r}^{y,0}$ and $\mathcal{D}_{2,r}^{y,0}$ replaced by $\mathcal{C}_5^y$ and $\mathcal{D}_{5,s}^y$, respectively. 
Since there is no fast transmission, we only have $V_f$ but not $U_f$, and all $U_f$ in Assumption \ref{Assumption interconnection} and \ref{Assumption Extra 2} should be replace by $V_f$.

 We define a composite Lyapunov function $U_5(\xi_5^y)\coloneqq (1-d) {U_s}(\xi_s) + d{V_f}(x,y)$ with $U_s$ defined by \eqref{eqn: definition of U_s} and $V_f$ come from Assumption \ref{Assumption Stable fast subsystem}.
% Along the same line as how we prove \eqref{eqn: U derivative}, by \eqref{eqn: Us flow}, \eqref{eqn: Assumption stable fast subsystem, Uf flow} and Assumption \ref{Assumption interconnection}, we can prove that there exists $\mu_2$, $\nu_3 >0$, a class-$\mathcal{K}$ function $\psi_4$, such that $U_5^\circ(\xi_5^y, F_5^y(\xi_5^y)) \leq - \mu_2 U(\xi_5^y) + 2 \nu_2$.
% %
%     % \begin{equation*}
%     %     U_5^\circ(\xi_5^y, F_5^y(\xi_5^y)) \leq - \mu_2 U(\xi_5^y) + 2 \nu_2.
%     % \end{equation*} 
% At jumps, similar to how we derive \eqref{eqn: U slow jump}, by \eqref{eqn: Us jump}, Assumption \ref{Assumption Vf at slow transmission}, we have
% \begin{equation*}
%     \begin{aligned}
%         &U_5(G_5^s(\xi_5^y)) \\
%         =& (1-d)U_s\big((x,h_s(\kappa_s,e_s), 0, \kappa_s + 1)\big) + d V_f(x,h_y(x,e_s,y)) \\
%         \leq& (1-d)U_s(\xi_s) + d V_f(x,y) +  d \big(V_f(x,h_y(x,e_s,y)) - V_f(x,y)\big)\\
%         \leq& U_5(\xi_5) + d\Big( \lambda_1 W_s^2(\kappa_s,e_s) + \lambda_2 \sqrt{W_s^2(\kappa_s,e_s) V_f(x,y)} \Big).\\
%         \leq& a_d U_5(\xi_5),
%     \end{aligned}
% \end{equation*}
% where $a_d$ is defined in \eqref{eqn: U slow jump}.
%
Then by following the same procedure as the proof of Theorem \ref{Theorem H_1}, we can prove $\mathcal{H}_5$ is SPAS w.r.t. $\mathcal{E}_5$.$\hfill\blacksquare$
