# Supplementary material for: Stabilization of singularly perturbed networked control systems over a single channel
Source: arXiv:2502.18768 source file (2025-02-26)
Supplement: Supplementary file 3 [file Appendix_Stable_slow_subsystem.tex]

\textbf{Proof of Corollary \ref{Corollary Stable slow subsystem}:} We define the composite Lyapunov function $U_6(x,\xi_f) \coloneqq V_s(x) + U_f(x,\xi_f)$, where $V_s$ comes from Assumption \ref{Assumption Stable slow subsystem} and $U_f$ is defined by \eqref{eqn: definition of U_f}. Similar to the proof of Theorem \ref{Theorem H_1}, there exist $\mathcal{K}_{\infty}$ functions $\underline{\alpha}_U$ and $\overline{\alpha}_{U}$, such that
\begin{equation*}
    \underline{\alpha}_U(\xi_6^y) \leq U(x,\xi_f) \leq  \overline{\alpha}_U(\xi_6^y).
\end{equation*}

Along the same line as how we prove \eqref{eqn: No disturbance U derivative}, by \eqref{eqn: Uf flow}, \eqref{eqn: Assumption stable slow subsystem, Us flow} and Assumption \ref{Assumption interconnection}, we can prove that for any $\epsilon \in (0,\epsilon^*)$, there exists a positive definite function $\rho_6$, such that
    \begin{equation*}
        U_6^\circ(\xi_6^y, F_6^y(\xi_6^y, \cyan{\epsilon})) \leq - \rho_6\left( |\xi_6^y|_{\mathcal{E}_6^y} \right),
    \end{equation*} 
where $\epsilon^*  = \tfrac{a_1 a_2}{a_1b_3 + b_1b_2}$.

At fast transmissions, by the definition of $U_6$ and the inequality \eqref{eqn: Us jump}, we have
\begin{equation*}
    \begin{aligned}
        U_6(G_{6,f}^y(\xi_6^y)) &= (1-d) V_s(x) + d U_f(G_{6,f}^y(\xi_6^y)) \\
        & \leq (1-d) V_s(x) + d U_f(\xi_6^y) \\
        & \leq U_6(\xi_6^y).
    \end{aligned}
\end{equation*}

We remind that $j$ denotes the total number of transmissions. By \eqref{eqn: Stefan miati} we have $j \leq \tfrac{t}{\tau_{\text{miati}}} + 1$. Then for any $t+j \geq T$, we have $t \geq T - \tfrac{t}{\tau_{\text{miati}}} - 1$, and by rearranging, we get
\begin{equation*}
    t \geq \frac{\tau_{\text{miati}}}{\tau_{\text{miati}} + 1} (T - 1).
\end{equation*}
By considering the Lyapunov function during flow, at fast jumps and the inequality above, we can conclude that $\mathcal{H}_6^y$ is uniformly globally pre-asymptotically stable (UGpAS) w.r.t. $\mathcal{E}_6^y$ according to \cite[Proposition 3.27]{gosate12}.

For same reason as in the proof of Theorem \ref{Theorem H_1}, exist a class $\mathcal{K}$ function $\zeta_6$ such that $|\overline{H}(x)| \leq \zeta_6(|x|)$ for all $x \in \mathbb{R}^{n_x}$. Consequently, the map $y = z - \overline{H}(x)$ is stability preserving \cite[pp. 450]{nonlinear_systems_Khalil}, which implies $\mathcal{H}_6$ is also UGpAS w.r.t. $\mathcal{E}$. Finally, by following the same steps as the proof of Theorem \ref{Theorem H_1}, i.e., containment \cite[Proposition 3.32]{gosate12} and completeness of solution, we can prove that $\mathcal{H}_6$ is UGAS w.r.t. $\mathcal{E}$.  $\hfill\blacksquare$
