# Supplementary material for: Stabilization of singularly perturbed networked control systems over a single channel
Source: arXiv:2502.18768 source file (2025-02-26)
Supplement: Supplementary file 4 [file Appendix_Stefan.tex]

\newpage
\textbf{Proof of Corollary \ref{Corollary Stefan Timer}:}
We will use the same Lyapunov functions as in the proof of Theorem \ref{Theorem H_1}, that is $U(\xi_s, \xi_f)\coloneqq (1-d) {U_s}(\xi_s) + d{U_f}(\xi_s,\xi_f)$ with $U_s$ and $U_f$ come from Lemma \ref{Lemma MATI}. Then we can prove that, there exist $\underline{\alpha}_U, \overline{\alpha}_U \in \mathcal{K}_{\infty}$, such that the sandwich bound \eqref{eqn: No disturbance U sandwich bound} holds for all $\xi^y \in \mathcal{C}_4^{y,\epsilon} \cup \mathcal{D}_{4,s}^{y,\epsilon} \cup \mathcal{D}_{4,f}^{y,\epsilon} $.

\emph{\underline{During flow}:} Along the same line as the proof of \eqref{eqn: U derivative with repect to xi}, We can proof that for all $\xi^y \in \mathcal{C}_4^{y,\epsilon}$ and $\epsilon \in (0, \epsilon^*)$, there exist a positive definite function $\rho$ such that the inequality below holds.
\begin{equation*}
    U^\circ(\xi^y, F^y(\xi^y, \cyan{\epsilon})) \leq - \rho(|\xi^y|_{\mathcal{E}^y}).
\end{equation*}

\emph{\underline{During jump}:} 
\red{At each slow jump, by definition of $U$, $G_{4,s}^y$ and inequality \eqref{eqn: Us jump}, 
\begin{equation*}
    \begin{aligned}
    U&(G_{4,s}^y(\xi^y)) \\
    =& (1-d){U_s}\big((x,h_s(\kappa_s, e_s), 0, \kappa_s+1)\big) + d{U_f}(G_{4,s}^y) \\
    \leq& (1-d)U_s(\xi_s) + d \big(V_f(x,h_y(x,e_s,y)) \\
        &+ \gamma_f \phi_f(\tau) W_f^2(\kappa_f,e_f) \big) \\
    =& U(\xi^y) + d \big(V_f(x,h_y(x,e_s,y)) - V_f(x,y)\big).
    \end{aligned}
\end{equation*}
By \eqref{eqn: Vf slow jump}, we have that for any $\xi$ in compact set $\Omega$, there exist a positive real number $L^\Omega$ such that
\begin{equation*}
    \begin{aligned}
        &U(G_{4,s}^y(\xi^y)) \\
        \leq& U(\xi^y) + d \overline{\alpha}_{V_f}\big( (1+L^\Omega)|\xi^y| \big) \\
        \leq& U(\xi^y) + d \overline{\alpha}_{V_f}\big( (1+L^\Omega)\underline{\alpha}_U^{-1}(U(\xi^y)) \big) \\
        \eqqcolon& \alpha_{4,s}^{L^\Omega} (U(\xi^y))
    \end{aligned}
\end{equation*}
}

At each fast jump, the jump map $G_{4,f}^y$ of $\mathcal{H}_4^y$ is equivalent to $G_s^y$. Then by following the procedure we derive \eqref{eqn: U fast update}, we can get
\begin{equation}
    U(G_{4,f}^y(\xi^y)) \leq U(\xi^y).
\end{equation}

We have obtained the conditions on Lyapunov function $U$ during flow, at slow transmissions and at fast transmissions, we can then prove Corollary \ref{Corollary Stefan Timer} by following the same procedure as the proof of Theorem \ref{Theorem H_1}. $\hfill\blacksquare$
